# Supplementary material for: Commuting Magic Square Matrices
Source: arXiv:2009.03499 ancillary file (2020-09-08)
Supplement: Supplementary file 1 [file Ultra25s.pdf]

|     |     |     |     |     |     |     |     |     |     |     |     |     |     |     |     |     |     |     |     |     |     |     |     |     |
|-----|-----|-----|-----|-----|-----|-----|-----|-----|-----|-----|-----|-----|-----|-----|-----|-----|-----|-----|-----|-----|-----|-----|-----|-----|
| 624 | 602 | 605 | 613 | 616 | 74  | 52  | 55  | 63  | 66  | 149 | 127 | 130 | 138 | 141 | 349 | 327 | 330 | 338 | 341 | 424 | 402 | 405 | 413 | 416 |
| 610 | 618 | 621 | 604 | 607 | 60  | 68  | 71  | 54  | 57  | 135 | 143 | 146 | 129 | 132 | 335 | 343 | 346 | 329 | 332 | 410 | 418 | 421 | 404 | 407 |
| 601 | 609 | 612 | 615 | 623 | 51  | 59  | 62  | 65  | 73  | 126 | 134 | 137 | 140 | 148 | 326 | 334 | 337 | 340 | 348 | 401 | 409 | 412 | 415 | 423 |
| 617 | 620 | 603 | 606 | 614 | 67  | 70  | 53  | 56  | 64  | 142 | 145 | 128 | 131 | 139 | 342 | 345 | 328 | 331 | 339 | 417 | 420 | 403 | 406 | 414 |
| 608 | 611 | 619 | 622 | 600 | 58  | 61  | 69  | 72  | 50  | 133 | 136 | 144 | 147 | 125 | 333 | 336 | 344 | 347 | 325 | 408 | 411 | 419 | 422 | 400 |
| 274 | 252 | 255 | 263 | 266 | 474 | 452 | 455 | 463 | 466 | 549 | 527 | 530 | 538 | 541 | 124 | 102 | 105 | 113 | 116 | 199 | 177 | 180 | 188 | 191 |
| 260 | 268 | 271 | 254 | 257 | 460 | 468 | 471 | 454 | 457 | 535 | 543 | 546 | 529 | 532 | 110 | 118 | 121 | 104 | 107 | 185 | 193 | 196 | 179 | 182 |
| 251 | 259 | 262 | 265 | 273 | 451 | 459 | 462 | 465 | 473 | 526 | 534 | 537 | 540 | 548 | 101 | 109 | 112 | 115 | 123 | 176 | 184 | 187 | 190 | 198 |
| 267 | 270 | 253 | 256 | 264 | 467 | 470 | 453 | 456 | 464 | 542 | 545 | 528 | 531 | 539 | 117 | 120 | 103 | 106 | 114 | 192 | 195 | 178 | 181 | 189 |
| 258 | 261 | 269 | 272 | 250 | 458 | 461 | 469 | 472 | 450 | 533 | 536 | 544 | 547 | 525 | 108 | 111 | 119 | 122 | 100 | 183 | 186 | 194 | 197 | 175 |
| 49  | 27  | 30  | 38  | 41  | 249 | 227 | 230 | 238 | 241 | 324 | 302 | 305 | 313 | 316 | 399 | 377 | 380 | 388 | 391 | 599 | 577 | 580 | 588 | 591 |
| 35  | 43  | 46  | 29  | 32  | 235 | 243 | 246 | 229 | 232 | 310 | 318 | 321 | 304 | 307 | 385 | 393 | 396 | 379 | 382 | 585 | 593 | 596 | 579 | 582 |
| 26  | 34  | 37  | 40  | 48  | 226 | 234 | 237 | 240 | 248 | 301 | 309 | 312 | 315 | 323 | 376 | 384 | 387 | 390 | 398 | 576 | 584 | 587 | 590 | 598 |
| 42  | 45  | 28  | 31  | 39  | 242 | 245 | 228 | 231 | 239 | 317 | 320 | 303 | 306 | 314 | 392 | 395 | 378 | 381 | 389 | 592 | 595 | 578 | 581 | 589 |
| 33  | 36  | 44  | 47  | 25  | 233 | 236 | 244 | 247 | 225 | 308 | 311 | 319 | 322 | 300 | 383 | 386 | 394 | 397 | 375 | 583 | 586 | 594 | 597 | 575 |
| 449 | 427 | 430 | 438 | 441 | 524 | 502 | 505 | 513 | 516 | 99  | 77  | 80  | 88  | 91  | 174 | 152 | 155 | 163 | 166 | 374 | 352 | 355 | 363 | 366 |
| 435 | 443 | 446 | 429 | 432 | 510 | 518 | 521 | 504 | 507 | 85  | 93  | 96  | 79  | 82  | 160 | 168 | 171 | 154 | 157 | 360 | 368 | 371 | 354 | 357 |
| 426 | 434 | 437 | 440 | 448 | 501 | 509 | 512 | 515 | 523 | 76  | 84  | 87  | 90  | 98  | 151 | 159 | 162 | 165 | 173 | 351 | 359 | 362 | 365 | 373 |
| 442 | 445 | 428 | 431 | 439 | 517 | 520 | 503 | 506 | 514 | 92  | 95  | 78  | 81  | 89  | 167 | 170 | 153 | 156 | 164 | 367 | 370 | 353 | 356 | 364 |
| 433 | 436 | 444 | 447 | 425 | 508 | 511 | 519 | 522 | 500 | 83  | 86  | 94  | 97  | 75  | 158 | 161 | 169 | 172 | 150 | 358 | 361 | 369 | 372 | 350 |
| 224 | 202 | 205 | 213 | 216 | 299 | 277 | 280 | 288 | 291 | 499 | 477 | 480 | 488 | 491 | 574 | 552 | 555 | 563 | 566 | 24  | 2   | 5   | 13  | 16  |
| 210 | 218 | 221 | 204 | 207 | 285 | 293 | 296 | 279 | 282 | 485 | 493 | 496 | 479 | 482 | 560 | 568 | 571 | 554 | 557 | 10  | 18  | 21  | 4   | 7   |
| 201 | 209 | 212 | 215 | 223 | 276 | 284 | 287 | 290 | 298 | 476 | 484 | 487 | 490 | 498 | 551 | 559 | 562 | 565 | 573 | 1   | 9   | 12  | 15  | 23  |
| 217 | 220 | 203 | 206 | 214 | 292 | 295 | 278 | 281 | 289 | 492 | 495 | 478 | 481 | 489 | 567 | 570 | 553 | 556 | 564 | 17  | 20  | 3   | 6   | 14  |
| 208 | 211 | 219 | 222 | 200 | 283 | 286 | 294 | 297 | 275 | 483 | 486 | 494 | 497 | 475 | 558 | 561 | 569 | 572 | 550 | 8   | 11  | 19  | 22  | 0   |

**Order-25 Ultra Magic Square Matrix A**  
**Commutates with Matrix B**

|     |     |     |     |     |     |     |     |     |     |     |     |     |     |     |     |     |     |     |     |     |     |     |     |     |
|-----|-----|-----|-----|-----|-----|-----|-----|-----|-----|-----|-----|-----|-----|-----|-----|-----|-----|-----|-----|-----|-----|-----|-----|-----|
| 624 | 74  | 149 | 349 | 424 | 602 | 52  | 127 | 327 | 402 | 605 | 55  | 130 | 330 | 405 | 613 | 63  | 138 | 338 | 413 | 616 | 66  | 141 | 341 | 416 |
| 274 | 474 | 549 | 124 | 199 | 252 | 452 | 527 | 102 | 177 | 255 | 455 | 530 | 105 | 180 | 263 | 463 | 538 | 113 | 188 | 266 | 466 | 541 | 116 | 191 |
| 49  | 249 | 324 | 399 | 599 | 27  | 227 | 302 | 377 | 577 | 30  | 230 | 305 | 380 | 580 | 38  | 238 | 313 | 388 | 588 | 41  | 241 | 316 | 391 | 591 |
| 449 | 524 | 99  | 174 | 374 | 427 | 502 | 77  | 152 | 352 | 430 | 505 | 80  | 155 | 355 | 438 | 513 | 88  | 163 | 363 | 441 | 516 | 91  | 166 | 366 |
| 224 | 299 | 499 | 574 | 24  | 202 | 277 | 477 | 552 | 2   | 205 | 280 | 480 | 555 | 5   | 213 | 288 | 488 | 563 | 13  | 216 | 291 | 491 | 566 | 16  |
| 610 | 60  | 135 | 335 | 410 | 618 | 68  | 143 | 343 | 418 | 621 | 71  | 146 | 346 | 421 | 604 | 54  | 129 | 329 | 404 | 607 | 57  | 132 | 332 | 407 |
| 260 | 460 | 535 | 110 | 185 | 268 | 468 | 543 | 118 | 193 | 271 | 471 | 546 | 121 | 196 | 254 | 454 | 529 | 104 | 179 | 257 | 457 | 532 | 107 | 182 |
| 35  | 235 | 310 | 385 | 585 | 43  | 243 | 318 | 393 | 593 | 46  | 246 | 321 | 396 | 596 | 29  | 229 | 304 | 379 | 579 | 32  | 232 | 307 | 382 | 582 |
| 435 | 510 | 85  | 160 | 360 | 443 | 518 | 93  | 168 | 368 | 446 | 521 | 96  | 171 | 371 | 429 | 504 | 79  | 154 | 354 | 432 | 507 | 82  | 157 | 357 |
| 210 | 285 | 485 | 560 | 10  | 218 | 293 | 493 | 568 | 18  | 221 | 296 | 496 | 571 | 21  | 204 | 279 | 479 | 554 | 4   | 207 | 282 | 482 | 557 | 7   |
| 601 | 51  | 126 | 326 | 401 | 609 | 59  | 134 | 334 | 409 | 612 | 62  | 137 | 337 | 412 | 615 | 65  | 140 | 340 | 415 | 623 | 73  | 148 | 348 | 423 |
| 251 | 451 | 526 | 101 | 176 | 259 | 459 | 534 | 109 | 184 | 262 | 462 | 537 | 112 | 187 | 265 | 465 | 540 | 115 | 190 | 273 | 473 | 548 | 123 | 198 |
| 26  | 226 | 301 | 376 | 576 | 34  | 234 | 309 | 384 | 584 | 37  | 237 | 312 | 387 | 587 | 40  | 240 | 315 | 390 | 590 | 48  | 248 | 323 | 398 | 598 |
| 426 | 501 | 76  | 151 | 351 | 434 | 509 | 84  | 159 | 359 | 437 | 512 | 87  | 162 | 362 | 440 | 515 | 90  | 165 | 365 | 448 | 523 | 98  | 173 | 373 |
| 201 | 276 | 476 | 551 | 1   | 209 | 284 | 484 | 559 | 9   | 212 | 287 | 487 | 562 | 12  | 215 | 290 | 490 | 565 | 15  | 223 | 298 | 498 | 573 | 23  |
| 617 | 67  | 142 | 342 | 417 | 620 | 70  | 145 | 345 | 420 | 603 | 53  | 128 | 328 | 403 | 606 | 56  | 131 | 331 | 406 | 614 | 64  | 139 | 339 | 414 |
| 267 | 467 | 542 | 117 | 192 | 270 | 470 | 545 | 120 | 195 | 253 | 453 | 528 | 103 | 178 | 256 | 456 | 531 | 106 | 181 | 264 | 464 | 539 | 114 | 189 |
| 42  | 242 | 317 | 392 | 592 | 45  | 245 | 320 | 395 | 595 | 28  | 228 | 303 | 378 | 578 | 31  | 231 | 306 | 381 | 581 | 39  | 239 | 314 | 389 | 589 |
| 442 | 517 | 92  | 167 | 367 | 445 | 520 | 95  | 170 | 370 | 428 | 503 | 78  | 153 | 353 | 431 | 506 | 81  | 156 | 356 | 439 | 514 | 89  | 164 | 364 |
| 217 | 292 | 492 | 567 | 17  | 220 | 295 | 495 | 570 | 20  | 203 | 278 | 478 | 553 | 3   | 206 | 281 | 481 | 556 | 6   | 214 | 289 | 489 | 564 | 14  |
| 608 | 58  | 133 | 333 | 408 | 611 | 61  | 136 | 336 | 411 | 619 | 69  | 144 | 344 | 419 | 622 | 72  | 147 | 347 | 422 | 600 | 50  | 125 | 325 | 400 |
| 258 | 458 | 533 | 108 | 183 | 261 | 461 | 536 | 111 | 186 | 269 | 469 | 544 | 119 | 194 | 272 | 472 | 547 | 122 | 197 | 250 | 450 | 525 | 100 | 175 |
| 33  | 233 | 308 | 383 | 583 | 36  | 236 | 311 | 386 | 586 | 44  | 244 | 319 | 394 | 594 | 47  | 247 | 322 | 397 | 597 | 25  | 225 | 300 | 375 | 575 |
| 433 | 508 | 83  | 158 | 358 | 436 | 511 | 86  | 161 | 361 | 444 | 519 | 94  | 169 | 369 | 447 | 522 | 97  | 172 | 372 | 425 | 500 | 75  | 150 | 350 |
| 208 | 283 | 483 | 558 | 8   | 211 | 286 | 486 | 561 | 11  | 219 | 294 | 494 | 569 | 19  | 222 | 297 | 497 | 572 | 22  | 200 | 275 | 475 | 550 | 0   |

## Order-25 Ultra Magic Square Matrix B

Commutates with Matrix A

## Definition of an Ultra Magic Square:

In an order- $n$  square the numbers  $0, 1, \dots, n^2 - 1$  occur once and only once.

The numbers in each row and column sum to the index  $m$ .

The numbers along each diagonal, including broken ones in both directions, sum to  $m$ .

The sum of every pair of elements symmetric about the center equals the index  $r$ .

In an odd-order square the center element equals  $r/2$ .

For an order- $n$  square  $m$  and  $r$  are given by

$$m = n(n^2 - 1)/2,$$

$$r = n^2 - 1.$$

For an order-25 square

$$m = 7800,$$

$$r = 624.$$

The two squares shown were constructed by compounding the order-five square:

Knight's move:

|   |   |   |   |   |
|---|---|---|---|---|
| 4 | 2 | 0 | 3 | 1 |
| 0 | 3 | 1 | 4 | 2 |
| 1 | 4 | 2 | 0 | 3 |
| 2 | 0 | 3 | 1 | 4 |
| 3 | 1 | 4 | 2 | 0 |

+ 5

Transpose:

|   |   |   |   |   |
|---|---|---|---|---|
| 4 | 0 | 1 | 2 | 3 |
| 2 | 3 | 4 | 0 | 1 |
| 0 | 1 | 2 | 3 | 4 |
| 3 | 4 | 0 | 1 | 2 |
| 1 | 2 | 3 | 4 | 0 |

=

Ultra Magic:

|    |    |    |    |    |
|----|----|----|----|----|
| 24 | 2  | 5  | 13 | 16 |
| 10 | 18 | 21 | 4  | 7  |
| 1  | 9  | 12 | 15 | 23 |
| 17 | 20 | 3  | 6  | 14 |
| 8  | 11 | 19 | 22 | 0  |
